# Supplementary material for: A Generalised Inverse Reinforcement Learning Framework
Source: arXiv:2105.11812 source file (2021-05-25)
Supplement: Supplementary file 1 [file off_policy_data_augmentation.tex]

\section{Off policy data augmentation}
\label{A:off_policy_idle}
    TBD.
    
    The idea is to decompose the problem into learning a classifier\footnote{{\color{cyan} je reflechis encore à un bon symbol interpretable pour le classifieur}} $C^*$ of this distribution and then learning a generator \hbox{$G:(s)\in\mathcal{S}\rightarrow (s_+,a_+)\in\mathcal{S}\times\mathcal{A}$} that maximises $P_{\pi}^\eta(G(s)|s)$ using a Generative Adversarial Network (GAN)-like approach. For this purpose, notice that $P_{\pi}^\eta$ can be re-written as: 
    \begin{equation*}
        \begin{array}{ll}
            P_{\pi}^\eta(s_+,a_+|s) = p(s_+,a_+)\frac{C^*(s_+,a_+|s)}{1-C^*(s_+,a_+|s)} \quad \textit{where} \quad C^*(s_+,a_+|s) = \frac{P_{\pi}^\eta(s_+,a_+|s)}{P_{\pi}^\eta(s_+,a_+|s) + p(s_+,a_+)} \\
        \end{array}
    \end{equation*}
    where the marginal future state distribution defined as:
    \begin{align*}
        p(s_+,a_+) := \int_{s_0,a_0} \hspace{-0.5cm} p_0(s_0)\pi(a_0|s_0) \int_{s,a}\hspace{-0.2cm}\rho_\pi(s,a|s_0,a_0)P_{\pi}^\eta(s_+,a_+|s,a)
    \end{align*}
    Given an on-policy data set of trajectories, a tractable approach to learn the classifier $C^*$ is to optimise the following loss function\cite{Clearning} :  
    \begin{align*}
        \mathcal{L}(C) &=  \mathbb{E}\big[ (1-\gamma) \log C(s_{t+1},a_{t+1}|s_t,a_t) +  \lfloor w \rfloor \log C(s_+,a_+|s_t,a_t) +  \log (1-C(s_+,a_+|s_t,a_t)) \big] 
    \end{align*}
    where the expectation is taken with respect to the marginal for $(s_+,a_+,s_t)$ and to the horizon distribution $\eta$ for $k$. and such that:
    \begin{align*}
        w = \frac{C(s_+,a_+|s_{t+1},a_{t+1})}{1-C(s_+,a_+|s_{t+1},a_{t+1})} \quad \textit{and} \quad C^* = \argmin_{C\in[0,1]^{\mathcal{S}\times\mathcal{A}\times\mathcal{S}}} \mathcal{L}(C) 
    \end{align*}
    
    In the context of IRL problems, the expert trajectories are by construction an on-policy data set. This guarantees the feasibility of learning such classifier for the expert policy.
    
    However, in order to learn $P_{\pi}^{\eta}$, it is not sufficient to maximise the classifier's log-probability as it does not take into account the marginal state action distribution. 
    To circumvent this issue we propose to solve a game between a discriminator $D: (\mathcal{S}\times\mathcal{A}\times\mathcal{S})\to[0,1]$ and a generator $G$. The goal of the generator $G$ is to produce future state like samples while the discriminator $D$ aims to identify true samples from generated ones. 
    We propose the following score functions for the game:
    \begin{align}
    \begin{split}
        V_{\textit{off}}(D,G) = & \mathbb{E}\big[ \frac{C^*(s_+,a_+|s)}{1-C^*(s_+,a_+|s)} \log(D(s_+,a_+|s)) + \log(1-D(G(s)|s)) \big] 
    \end{split}
    \label{idle_game}
    \end{align}
    where the expectation is taken with respect to the marginal for $(s_+,a_+,s)$. Solving this game approximates $P_{\pi}^{\eta}$.
    The generator maximises $f_{gen}(G|D)$: the likelihood of the generated samples given a discriminator, while $D$ maximises the binary cross entropy $f_{disc}(D|G)$ in order to separate true samples from generated ones.
    \begin{proposition}
        $(\Tilde{D}=\frac{1}{2},\Tilde{G}=P_{\pi}^{\eta})$ is a Nash-equilibrium of the following zero-game:
        \begin{align}
            D^* = \argmin_D V_{\textit{off}}(D,G) \; ; \;
            G^* = \argmax_G V_{\textit{off}}(D,G)
        \end{align}
    \end{proposition}
    \subsubsection*{Proof:}
        The proof relies on observing that we can estimate expectations that use the future state distribution by sampling from the marginal and then weighting those samples by an importance weight. In fact:
        \begin{align}
            V_{\textit{off}}(D,G) = & \mathbb{E}\Big[ \frac{C^*(s_+,a_+|s)}{1-C^*(s_+,a_+|s)} \log(D(s_+,a_+|s)) + \log(1-D(G(s)|s)) \Big] \\
            = & \int_{s,a,s_+,a_+} \hspace{-1cm} p(s,a) p(s_{+},a_{+}) \frac{C^*(s_+,a_+|s)}{1-C^*(s_+,a_+|s)} \log(D(s_+,a_+|s))  + \int_{s,a} p(s,a) \log(1-D(G(s)|s)) \\
            = & \int_{s,a,s_+,a_+} \hspace{-1cm} p(s,a) P_\pi^\eta(s_{+},a_{+}|s) \log(D(s_+,a_+|s))  + \int_{s,a} p(s,a) \log(1-D(G(s)|s)) \\
            = & \int_{s,a} p(s,a) \mathbb{E}_{\substack{s_{+},a_{+}\sim P_\pi^\eta(s_{+},a_{+}|s) \\ s_{g},a_{g}\sim G(s)}} \Big[ \log(D(s_+,a_+|s)) + \log(1-D(s_{g},a_{g}|s)) \Big]
        \end{align}
        This is the loss function used by conditional generative adversarial neural networks, which minimum w.r.t the discriminator is achieved for the optimal Bayes classifier $D^*$:
        \begin{align}
            D^*(s,a|s_0) = \frac{P_\pi^\eta(s,a|s_0)}{P_\pi^\eta(s,a|s_0) + P_{G}(s,a|s_0)}
        \end{align}
        where $P_{G}(s,a|s_0)$ is the probability of generating $(s,a)$ using the generator $G$.
        From this, we can re-write the optimal generator's loss against an infinite capacity discriminator as:
        \begin{align}
            V_{\textit{off}}(D^*,G) & = D_{KL}(P_\pi^\eta(s,a|s_0) \| \frac{P_\pi^\eta(s,a|s_0)}{P_\pi^\eta(s,a|s_0) + P_{G}(s,a|s_0)}) + D_{KL}(P_{G}(s,a|s_0) \| \frac{P_\pi^\eta(s,a|s_0)}{P_\pi^\eta(s,a|s_0) + P_{G}(s,a|s_0)}) - \log(4) \\
            & = 2D_{JSC}(P_{G}(s,a|s_0) \| P_\pi^\eta(s,a|s_0)) - \log(4)
        \end{align}
        where $D_{KL}$ is the KL divergence, and $D_{JSC}$ is the Jenson-Shannon divergence. This yields a global minimum when $G^*$ achieves:
        \begin{align}
            P_{G^*}(s,a|s_0)=P_\pi^\eta(s,a|s_0).
        \end{align}
    
    A practical implication of this proposition is an algorithm that constructs good approximation of $P_{\pi}^{\eta}$ that  is used as a subroutine of $\GIRL$:
    
    \begin{algorithm}
            \caption{Idle (a $\gamma$-discounted future state generator)}\label{Idle}
            \begin{algorithmic}[1]
                \STATE {\bfseries Input:} Trajectories $\tau$, Classifier $C^*$, initial discriminator $D_{\phi_0}$ and initial generator $G_{\nu_0}$
                \FOR{$e \in [1, N]$}
                \STATE Sample state action $(S^+,A^+,S)\sim \tau$
                \STATE Sample $(S^+_G,A^+_G)\sim G_{\nu_i}(S)$
                \STATE Update the discriminator parameter $\phi_i$ to maximise: 
                $
                    \begin{array}{l}
                        \sum_{\substack{S,S^+,A^+}} \frac{C^*(s_+,a_+|s)}{1-C^*(s_+,a_+|s)} \log(D_{\phi_i}(s_+,a_+|s)) + \\
                        \sum_{\substack{S,S^+_G,A^+_G}} \frac{1-C^*(s_+,a_+|s)}{C^*(s_+,a_+|s)} \log(1-D_{\phi_i}(s_+,a_+|s))
                    \end{array}
                $
                 \STATE Update the generator parameter $\nu_i$ to maximise: 
                  $\quad\quad \sum_{\substack{S}} \log(D(G(s)|s))$
                \ENDFOR
                \STATE {\bfseries Return:} $(D_{\phi_N}, G_{\nu_N})$
            \end{algorithmic}
        \end{algorithm}
